# Supplementary material for: Flexible discrete space models of animal movement
Source: arXiv:1606.07986 source file (2016-06-26)
Supplement: Supplementary file 1 [file Appendix_A.pdf]

# Appendix A: Discrete Space Modeling of Northern Fur Seal Movement

In this appendix, we provide all code needed to replicate the analysis of the northern fur seal (NFS) movement path using a continuous-time Markov chain model for animal movement. In addition, we provide additional details on multiple imputation (Rubin 1987) and show that results from multiple imputation and the stacked weighted likelihood (SWL) proposed in Section 3.2 of the manuscript are nearly identical. This provides justification for using the SWL for movement data when paths need to be imputed between telemetry locations. The SWL is appealing because it allows any method which has been developed for Poisson regression to be applied to modeling movement within a CTMC framework.

We will follow the general framework proposed in Section 3.3

## 1. Collect telemetry data in the form of $\{(x_i, y_i, t_i),\ t_i = t_1, t_2, \ldots, t_K\}$.

We begin by loading the required R packages and reading in the NFS data, which is provided as part of the 'ctmcmove' package.

```
library(ctmcmove)
data(seal)
xyt=seal$locs[,3:1]
```

```
head(xyt)
```

```
##      longitude latitude datetime
## 1139  189.8883   57.243 36741.23
## 1140  189.9150   57.264 36741.29
## 1141  189.8970   57.252 36741.30
## 1142  190.3680   57.164 36741.62
## 1143  190.2510   57.468 36741.76
## 1144  190.6190   57.425 36741.87
```

```
xy=xyt[,-3]
x=xyt[,1]
y=xyt[,2]
t=xyt[,3]
set.seed(1337)
```

We then examine and plot the telemetry data:

```
plot(xyt[,1:2],type="b")
```

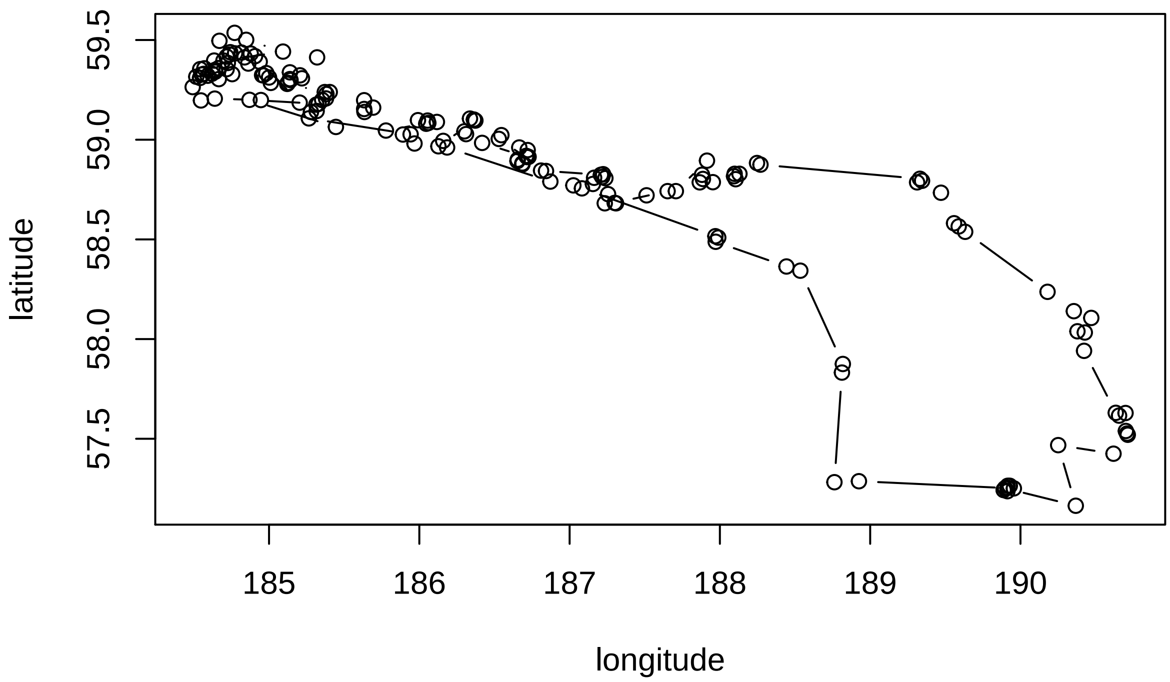


## 2. Collect and create covariate rasters

Next, we read in rasters related to environmental conditions encountered by the NFS. These rastes will both define the discrete support of the CTMC, and serve as covariates to help describe NFS movement behavior in different environments. The rasters are in the "seal" object in 'ctmcmove'

```
cov.df=seal$cov.df
str(cov.df)
```

```
## List of 1
##  $ X:'data.frame':   10000 obs. of  5 variables:
##   ..$ x  : num [1:10000] 184 184 184 184 184 ...
##   ..$ y  : num [1:10000] 56.7 56.7 56.7 56.7 56.7 ...
##   ..$ chA: num [1:10000] 1.19 0.924 0.744 0.709 0.733 ...
##   ..$ sst: num [1:10000] 9.07 10.35 10.27 10.43 9.98 ...
##   ..$ pro: num [1:10000] 853 821 823 849 886 ...
```

We have rasters for sea surface temperature (SST), chlorophyll A levels (chA), and net primary productivity (npp). Each is read in to R:

```
NN=sqrt(nrow(cov.df$X))
sst=matrix(seal$cov.df$X$sst,NN,byrow=TRUE)
sst=sst[NN:1,]
sst=raster(sst,xmn=min(seal$cov.df$X$x),xmx=max(seal$cov.df$X$x),
           ymn=min(seal$cov.df$X$y),ymx=max(seal$cov.df$X$y))


crs(sst)="+proj=longlat +datum=WGS84"
```

```r
chA=matrix(seal$cov.df$X$chA,NN,byrow=TRUE)
chA=chA[NN:1,]
chA=raster(chA,xmn=min(seal$cov.df$X$x),xmx=max(seal$cov.df$X$x),
           ymn=min(seal$cov.df$X$y),ymx=max(seal$cov.df$X$y))
crs(chA)="+proj=longlat +datum=WGS84"

pro=matrix(seal$cov.df$X$pro,NN,byrow=TRUE)
pro=pro[NN:1,]
npp=raster(pro,xmn=min(seal$cov.df$X$x),xmx=max(seal$cov.df$X$x),
           ymn=min(seal$cov.df$X$y),ymx=max(seal$cov.df$X$y))
crs(npp)="+proj=longlat +datum=WGS84"
```

We then create two additional rasters. The first is an "intercept", with all values equal to 1 (int), and the second is a raster of the great circle distance from each raster grid cell to the NFS rookery on the Pribilof Islands (d2r).

```r
int=sst
values(int) <- 1

d2r=int
rookery.cell=cellFromXY(int,xyt[1,1:2])
values(d2r)=NA
values(d2r)[rookery.cell]=0
d2r=distance(d2r)
```

We then stack them all together in a RasterStack object

```r
grad.stack=stack(sst,chA,npp,d2r)
names(grad.stack) <- c("sst","cha","npp","d2r")
plot(grad.stack)
```

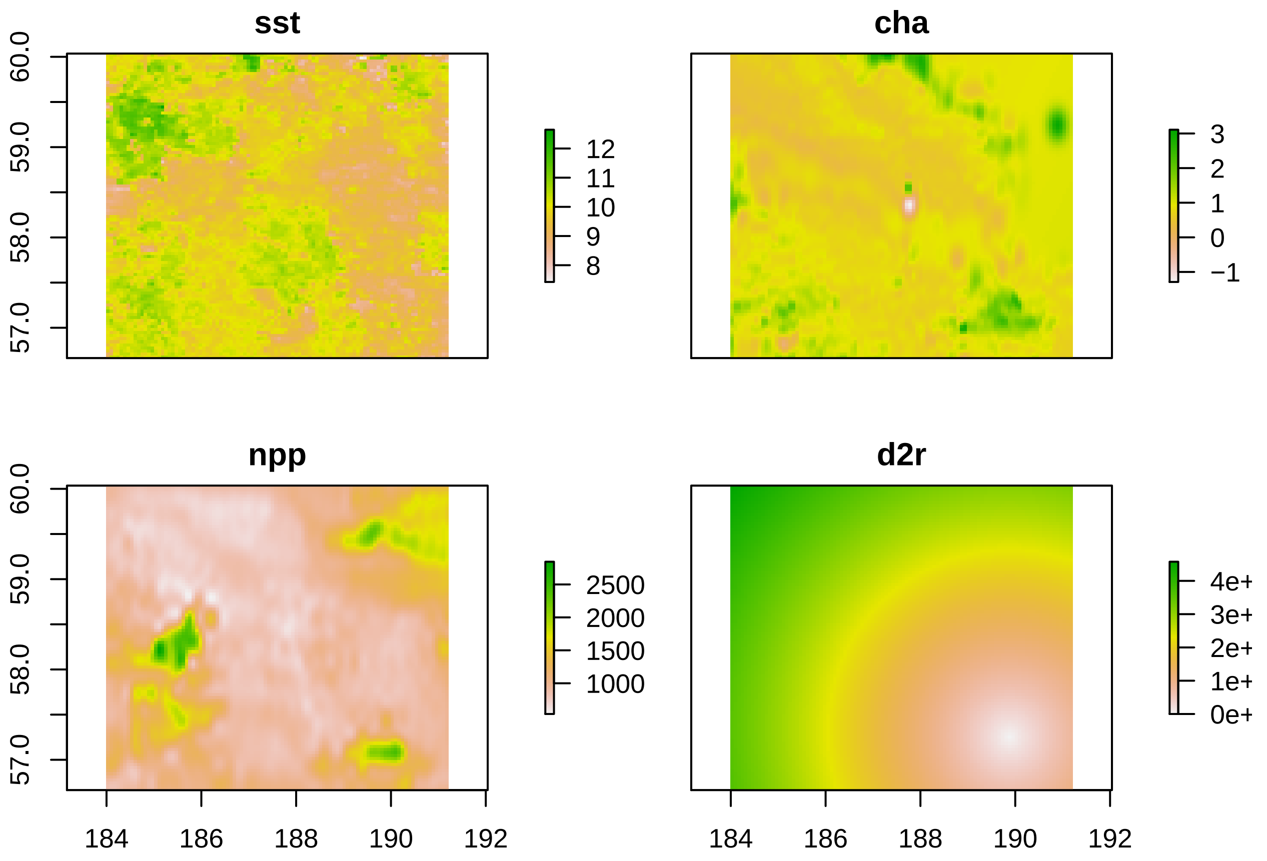


## 3. Impute $P$ continuous paths

We next fit the functional movement model (FMM) of Buderman et al., (2016) to the NFS telemetry data. Other continuous-time continuous-space movement models could be fit instead. An appealing alternative is the continuous-time correlated random walk (CTCRW) model of Johnson et al., (2008), which can be fit using the 'crawl' package in R.

To fit the FMM to the telemetry data, we first specify the knots for the B-spline basis expansion. Problems with fitting the FMM can often be fixed by varying the spacing of the knots. We also define the time-points at which we will sample the imputed path. For the NFS data, we impute the path at every minute. In general it will be helpful to impute the path at a temporal resolution fine enough that multiple time points are observed in most grid cells that the animal passes through.

```
## Define the knots of the spline expansion.
knots = seq(min(t),max(t),by=1/4)
## create B-spline basis vectors used to approximate the path
b=create.bspline.basis(c(min(t),max(t)),breaks=knots,norder=3)
## define the sequence of times on which to sample the imputed path
tpred=seq(min(t),max(t),by=1/24/60)
```

The 'ctmcmove' package contains code to fit the FMM and draw $P$ paths from the posterior predictive path distribution. We choose $P = 20$ here. In general, $P = 10$ imputations are often enough to obtain stable inference. When $P > 30$, results are often indistinguishable from full Bayesian inference carried out by imputing a new path at each iteration of an MCMC sampler.

```
P=20
out=mcmc.fmove(xy,t,b,tpred,QQ="CAR",n.mcmc=400,a=1,r=1,num.paths.save=P)
```

```
## 100  200  300  400
```

```
## plot 3 imputed paths
plot(xy,type="b")
points(out$pathlist[[1]]$xy,col="red",type="l")
points(out$pathlist[[2]]$xy,col="blue",type="l")
points(out$pathlist[[3]]$xy,col="green",type="l")
```

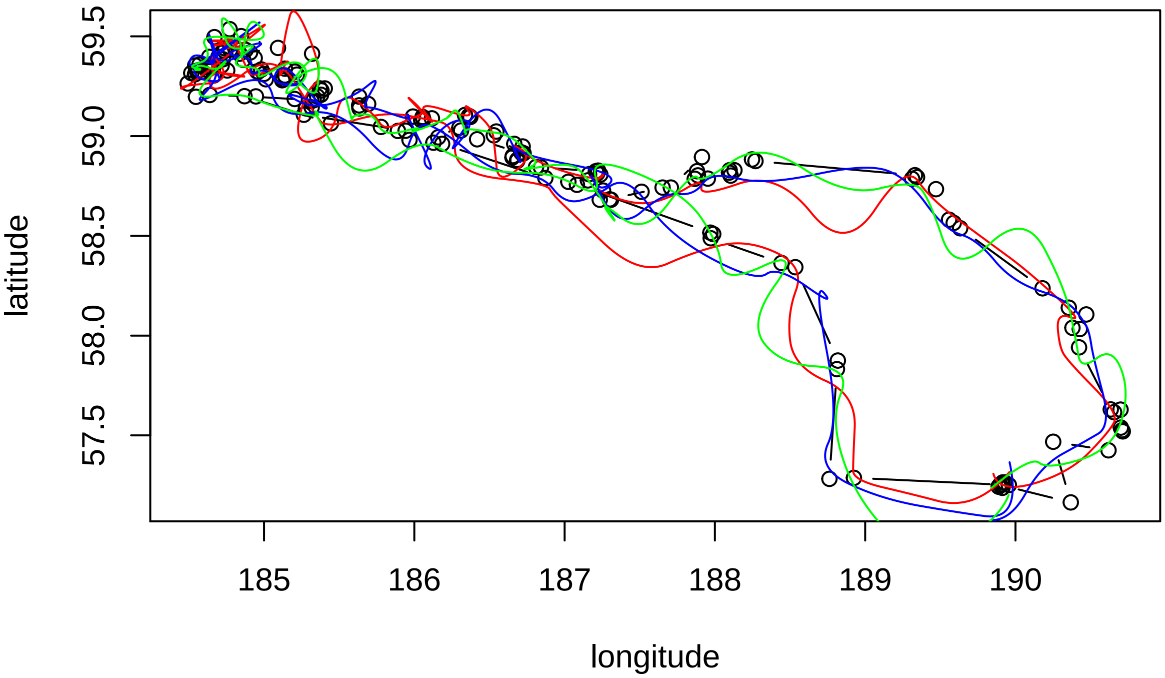


The imputed paths are smooth, and are at a fine enough resolution to show which raster cells may have been traversed in the NFS's path.

## 4. Discretize each path to obtain $P$ CTMC paths on the raster grid

Each quasi-continuous path can then be transformed into a discrete-space path on the raster grid using the `path2ctmc` function from 'ctmcmove'. The result is a list with entries corresponding to the embedded chain (the sequence of "cells" of the raster object that the path traverses), the residence time, and transition times of the CTMC.

```
path=out$pathlist[[1]]
ctmc=path2ctmc(path$xy,path$t,int)
str(ctmc)
```

```
## List of 3
##  $ ec         : num [1:481] 8082 8182 8282 8283 8284 ...
##  $ rt         : num [1:481] 0.00417 0.05139 0.04444 0.06458 0.04931 ...
##  $ trans.times: num [1:481] 36741 36741 36741 36741 36741 ...
```

# 5. Convert each CTMC path to data appropriate for a Poisson GLM likelihood by creating the auxiliary variables for each path

We next convert each CTMC path to data $(\mathbf{z}, \boldsymbol{\tau})^{(1)}, (\mathbf{z}, \boldsymbol{\tau})^{(2)}, \ldots, (\mathbf{z}, \boldsymbol{\tau})^{(P)}$ by creating

$$z_{tk} = \begin{cases} 1 & , \text{ if } k = c_{t+1} \\ 0 & , \text{ if } k \neq c_{t+1} \end{cases} . \tag{1}$$

for each grid cell in the embedded chain and each possible transition from that grid cell. This is accomplished using the `ctmc2glm' function in`ctmcmove'. This function additionally creates the motility covariates $m_{kl}$ and the gradients of the directional covariates $q_{pij} = \mathbf{e}'_{ij}\mathbf{g}_{pi}$ that are used in the loglinear model for the CTMC transition rates $\alpha_{ij}$.

$$\alpha_{ij} = \begin{cases} \exp\left\{\sum_{k=1}^{L} \delta_k m_{ki} + \sum_{p=1}^{P} \gamma_p \mathbf{e}'_{ij}\mathbf{g}_{pi}\right\} & , \text{ if } i \text{ and } j \text{ are neighbors} \\ 0 & , \text{ otherwise} \end{cases} . \tag{2}$$

The set of motility covariates is defined by one RasterStack object, with each layer in the RasterStack corresponding to a covariate, and the set of directional covariates is similarly defined by another RasterStack object. For this analysis, we will consider SST and the intercept for motility covariates, and all covariates (including SST) for directional covariates.

```
loc.stack=stack(int,sst)
names(loc.stack) <- c("Intercept","sst.loc")

glm.list=list()
glm.list[[1]]=ctmc2glm(ctmc,loc.stack,grad.stack)

str(glm.list)
```

```
## List of 1
##  $ :'data.frame':    1920 obs. of  14 variables:
##   ..$ z        : num [1:1920] 0 0 0 1 0 0 0 1 0 1 ...
##   ..$ Intercept: num [1:1920] 1 1 1 1 1 1 1 1 1 1 ...
##   ..$ sst.loc  : num [1:1920] 9.11 9.11 9.11 9.11 9.38 ...
##   ..$ sst      : num [1:1920] 7.54e-06 -7.54e-06 4.77e-05 -4.77e-05 1.37e-11 ...
##   ..$ cha      : num [1:1920] 5.64e-05 -5.64e-05 4.18e-05 -4.18e-05 4.82e-05 ...
##   ..$ npp      : num [1:1920] 0.00425 -0.00425 -0.00446 0.00446 0.00167 ...
##   ..$ d2r      : num [1:1920] -4.58e-17 4.58e-17 -7.48e-01 7.48e-01 -4.11e-17 ...
##   ..$ crw      : num [1:1920] 0 0 0 0 0 0 -1 1 0 0 ...
##   ..$ x.current: num [1:1920] 190 190 190 190 190 ...
##   ..$ y.current: num [1:1920] 57.3 57.3 57.3 57.3 57.3 ...
##   ..$ x.adj    : num [1:1920] 190 190 190 190 190 ...
##   ..$ y.adj    : num [1:1920] 57.3 57.3 57.4 57.3 57.3 ...
##   ..$ tau      : num [1:1920] 0.00417 0.00417 0.00417 0.00417 0.05139 ...
##   ..$ t        : num [1:1920] 36741 36741 36741 36741 36741 ...
```

The resulting data frame has the $z$ response variable, the residence time $\tau$ (tau), and a set of covariates. The motility covariates are given first, followed by the directional covariates and the autocovariate (crw). In addition, `ctmc2glm` also outputs the location of the current grid cell in the CTMC, the location of the neighboring grid cell to which the CTMC could transition next, and the time of the transition ($t$).

We now repeat this process for the other 19 imputed paths.

```
for(i in 2:P){
    path=out$pathlist[[i]]
    ctmc=path2ctmc(path$xy,path$t,int)
    glm.list[[i]]=ctmc2glm(ctmc,loc.stack,grad.stack)
}
```

Occasionally, an imputed continuous space path will transition directly through a "corner" of a grid cell, resulting in an impossibly-quick movement through one grid cell. These data points would essentially be outliers in the Poisson regression we will run, and we thus remove them.

```
for(i in 1:P){
    idx.0=which(glm.list[[i]]$tau<10^-5)
    if(length(idx.0)>0){
        glm.list[[i]]=glm.list[[i]][-idx.0,]
    }
    glm.list[[i]]$t=glm.list[[i]]$t-min(glm.list[[i]]$t)
}
```

# 6. Stack together the imputed paths

We then stack together the Poisson GLM-ready data from each path, as if they were independent observations.

```
glm.data=glm.list[[1]]
for(i in 2:P){
    glm.data=rbind(glm.data,glm.list[[i]])
}

str(glm.data)
```

```
## 'data.frame':    39660 obs. of  14 variables:
##  $ z        : num  0 0 0 1 0 0 0 1 0 1 ...
##  $ Intercept: num  1 1 1 1 1 1 1 1 1 1 ...
##  $ sst.loc  : num  9.11 9.11 9.11 9.11 9.38 ...
##  $ sst      : num  7.54e-06 -7.54e-06 4.77e-05 -4.77e-05 1.37e-11 ...
##  $ cha      : num  5.64e-05 -5.64e-05 4.18e-05 -4.18e-05 4.82e-05 ...
##  $ npp      : num  0.00425 -0.00425 -0.00446 0.00446 0.00167 ...
##  $ d2r      : num  -4.58e-17 4.58e-17 -7.48e-01 7.48e-01 -4.11e-17 ...
##  $ crw      : num  0 0 0 0 0 0 -1 1 0 0 ...
##  $ x.current: num  190 190 190 190 190 ...
##  $ y.current: num  57.3 57.3 57.3 57.3 57.3 ...
##  $ x.adj    : num  190 190 190 190 190 ...
##  $ y.adj    : num  57.3 57.3 57.4 57.3 57.3 ...
##  $ tau      : num  0.00417 0.00417 0.00417 0.00417 0.05139 ...
##  $ t        : num  0 0 0 0 0.0514 ...
```

# 7. Make inference on CTMC parameters using Poisson GLM software

We can then make inference on CTMC parameters by using Poisson GLM software, with each observation given a "weight" of $1/P$, and with $\tau$ being an offset. This corresponds to fitting the following Poisson

regression model:

$$z_{tk} \overset{iid}{\sim} \text{Pois}(\tau_t \alpha_{c_t k}), \quad t = 1, 2, \ldots, T; \quad k = 1, 2, \ldots, N \tag{3}$$

We show multiple approaches for estimating CTMC movement parameters under this paradigm.

## 7.1 Stacked Weighted Likelihood (SWL)

Inference under the SWL involves simply fitting the stacked GLM data from all $P$ imputed paths jointly, giving each observation a weight of $1/P$.

```
fit=glm(z~cha+npp+sst+crw+d2r+sst.loc,
        weights=rep(1/P,nrow(glm.data)),family="poisson",offset=log(tau),data=glm.data)
beta.hat.SWL=coef(fit)
beta.se.SWL=summary(fit)$coef[,2]
summary(fit)
```

```
##
## Call:
## glm(formula = z ~ cha + npp + sst + crw + d2r + sst.loc, family = "poisson",
##     data = glm.data, weights = rep(1/P, nrow(glm.data)), offset = log(tau))
##
## Deviance Residuals:
##      Min        1Q    Median        3Q       Max
## -0.77355  -0.14858  -0.09939  -0.01872   0.91288
##
## Coefficients:
##               Estimate Std. Error z value Pr(>|z|)
## (Intercept)  4.031e+00  5.283e-01   7.630 2.35e-14 ***
## cha         -7.610e+02  2.450e+03  -0.311    0.756
## npp          2.717e+00  5.144e+00   0.528    0.597
## sst         -1.027e+03  8.307e+02  -1.237    0.216
## crw          8.060e-01  6.885e-02  11.707  < 2e-16 ***
## d2r          1.026e-01  8.192e-02   1.252    0.210
## sst.loc     -2.408e-01  5.204e-02  -4.627 3.71e-06 ***
## ---
## Signif. codes:  0 '***' 0.001 '**' 0.01 '*' 0.05 '.' 0.1 ' ' 1
##
## (Dispersion parameter for poisson family taken to be 1)
##
##     Null deviance: 1760.9  on 39659  degrees of freedom
## Residual deviance: 1590.5  on 39653  degrees of freedom
## AIC: 2595.9
##
## Number of Fisher Scoring iterations: 6
```

From this we see that the NFS does not seem to be responding at all to gradients of SST, NPP, or chA. We have thus removed these covariates from the results presented in Section 4 of our manuscript. The 'sst.loc' covariate corresponds to treating SST as a motility covariate. As this is significantly less than zero, we could conclude that the NFS in general moves more slowly in regions of higher SST.

### 7.2 Multiple Imputation

Following Hanks et al., (2015), we next make inference using multiple imputation. This involves first fitting each path independently

```
glm.fits=list()
for(i in 1:P){
    glm.fits[[i]]=glm(z~cha+npp+sst+crw+d2r+sst.loc,
        family="poisson",offset=log(tau),data=glm.list[[i]])
}
```

and then getting point estimates and standard errors for all parameters using the combining rules of Rubin (1987). See Hanks et al., (2015) for details.

```
## get point estimates and se estimates using Rubin's MI combining rules
beta.hat.mat=integer()
beta.se.mat=integer()
for(i in 1:P){
    beta.hat.mat=rbind(beta.hat.mat,coef(glm.fits[[i]]))
    beta.se.mat=rbind(beta.se.mat,summary(glm.fits[[i]])$coef[,2])
}

beta.hat.mat
```

```
##       (Intercept)        cha         npp         sst       crw        d2r
##  [1,]    2.817915 -2353.8443  9.59926563    62.28985 2.8487486 0.12573064
##  [2,]    4.023657  -438.8246  3.90088471 -1793.21723 0.6307905 0.07800180
##  [3,]    5.085016  1042.1137 -0.92142933  -784.37145 0.7264329 0.08134997
##  [4,]    3.901352  1309.0473 -1.09752533 -1027.26339 0.7614293 0.12457309
##  [5,]    4.446739  1035.3942  2.14362582  -552.07646 0.6931744 0.09967207
##  [6,]    3.424915   373.3886 -2.36461279 -1656.79408 0.8095497 0.06079373
##  [7,]    4.160932 -1939.3709  2.16067274 -2973.44444 0.7761571 0.15540974
##  [8,]    2.518121  -864.9887  2.68018991  -962.86401 0.8174424 0.03034523
##  [9,]    4.349123 -1405.9489 -0.60769854 -1014.14424 0.7262710 0.13048010
## [10,]    3.405981  -620.7292 14.65885302  -298.37521 0.8692509 0.11379264
## [11,]    3.472406  -874.8115  5.59235616  -479.69332 0.7629428 0.15287644
## [12,]    3.614288  -857.4606 -0.01424927 -1372.25042 0.8200046 0.09149269
## [13,]    4.584758 -2095.8889  4.11421173  -959.20217 0.7775020 0.09754146
## [14,]    4.461525 -1890.2251  3.17780235  -707.59741 0.8039906 0.09336458
## [15,]    4.777929  -528.0297  5.21802288  -864.99411 0.6871624 0.11666318
## [16,]    4.496652 -2544.8940  7.00535343 -1776.67104 0.7479593 0.13413696
## [17,]    4.166092 -1151.9335  2.41300187  -347.10806 0.6154142 0.08029079
## [18,]    3.953119 -1292.7443  3.66763603 -1163.78758 0.7487378 0.10210630
## [19,]    4.119814 -1296.2007  2.45533929  -739.17056 0.7130346 0.06644614
## [20,]    4.164349   188.3003  2.10888849 -1459.06883 0.7471472 0.08914081
##           sst.loc
##  [1,] -0.26638349
##  [2,] -0.23496458
##  [3,] -0.34643146
##  [4,] -0.22463249
##  [5,] -0.28802942
##  [6,] -0.17286888
##  [7,] -0.25345190
```

```
##  [8,] -0.08964847
##  [9,] -0.26438582
## [10,] -0.18603755
## [11,] -0.18290148
## [12,] -0.20270257
## [13,] -0.29829015
## [14,] -0.28329550
## [15,] -0.31539806
## [16,] -0.27960023
## [17,] -0.24487387
## [18,] -0.23093172
## [19,] -0.24057255
## [20,] -0.25027575
```

```
beta.se.mat
```

```
##       (Intercept)      cha      npp      sst        crw        d2r
##  [1,]   0.5673843 2526.984 5.554618 789.2289 0.14146436 0.08302094
##  [2,]   0.5229697 2324.158 4.622697 878.3438 0.06730341 0.08321433
##  [3,]   0.5468810 2899.709 5.809886 902.7418 0.06950626 0.08326227
##  [4,]   0.5259370 2638.393 4.629871 855.8518 0.06792921 0.08306475
##  [5,]   0.5432085 2650.083 5.865659 899.8199 0.07101102 0.08643333
##  [6,]   0.4996223 2239.241 4.186288 802.7534 0.06629402 0.07812011
##  [7,]   0.5202298 3196.589 4.354460 834.5668 0.06912702 0.08272946
##  [8,]   0.5398783 2799.235 5.941322 782.4703 0.06785688 0.08045431
##  [9,]   0.5248281 2478.963 4.762553 844.0419 0.06656466 0.08098520
## [10,]   0.5261863 2312.621 6.341626 769.9689 0.07069221 0.08315951
## [11,]   0.5149223 2110.438 5.272347 807.2391 0.06823551 0.08264311
## [12,]   0.5369279 2245.550 7.512178 875.2763 0.06990770 0.08341267
## [13,]   0.5285943 2333.844 6.722693 843.9138 0.06950606 0.08285523
## [14,]   0.5250030 2046.227 4.430592 788.6748 0.06890106 0.08319470
## [15,]   0.5326194 2678.210 4.967229 910.7573 0.06927941 0.08415325
## [16,]   0.5262029 2461.861 5.166778 880.2985 0.06688326 0.08031441
## [17,]   0.5322643 2345.072 5.017452 824.6542 0.06548521 0.08005513
## [18,]   0.5316044 2442.606 5.333584 828.9110 0.06830058 0.08228245
## [19,]   0.5489324 2366.283 4.894274 812.8732 0.06569227 0.07989943
## [20,]   0.5239254 3172.158 5.583498 834.5465 0.06820174 0.08163713
##          sst.loc
##  [1,] 0.05514978
##  [2,] 0.05149149
##  [3,] 0.05420475
##  [4,] 0.05163082
##  [5,] 0.05377375
##  [6,] 0.04896187
##  [7,] 0.05113742
##  [8,] 0.05286269
##  [9,] 0.05163398
## [10,] 0.05191385
## [11,] 0.05052620
## [12,] 0.05269078
## [13,] 0.05245465
## [14,] 0.05182016
## [15,] 0.05274510
## [16,] 0.05178484
```

```
## [17,] 0.05264066
## [18,] 0.05228578
## [19,] 0.05410960
## [20,] 0.05130572
```

```
## E(beta) = E_paths(E(beta|path))
beta.hat.MI=apply(beta.hat.mat,2,mean)
beta.hat.MI
```

```
##   (Intercept)           cha           npp           sst           crw
##     3.9972341  -810.3825402     3.2945294 -1043.4902085     0.8541571
##           d2r       sst.loc
##     0.1012104    -0.2427838
```

```
## Var(beta) = E_paths(Var(beta|path))+Var_paths(E(beta|path))
beta.var.MI=apply(beta.se.mat^2,2,mean)+apply(beta.hat.mat,2,var)
beta.se.MI=sqrt(beta.var.MI)
```

## 7.3 Comparing MI and SWL

Multiple imputation is the premier method for inference in the presence of missing data. We show here that the SWL provides nearly identical inference to that obtained using multiple imputation. The benefit of the SWL approach is that it easly lends itself to penalized likelihood approaches, including AIC-based model selection or model averaging, LASSO and ridge regression, and genearlized additive models (GAMs), such as varying-coefficient models.

The following code plots the point estimates and standard errors obtained from multiple imputation and inference using the SWL. The results are nearly identical.

```
## standardize regression coefficients by multiplying by the SE of the X matrix
sds=apply(model.matrix(fit),2,sd)
sds[1]=1

## plot MI and SWL regression coefficients
par(mfrow=c(1,2))
plot(beta.hat.MI*sds,beta.hat.SWL*sds,main="(a) Coefficient Estimates",xlab="Weighted Likelihood Coeffi
abline(0,1,col="red")
plot(log(beta.se.MI),log(beta.se.SWL),main="(b) log(Standard Errors)",xlab="Weighted Likelihood log(SE)
abline(0,1,col="red")
```

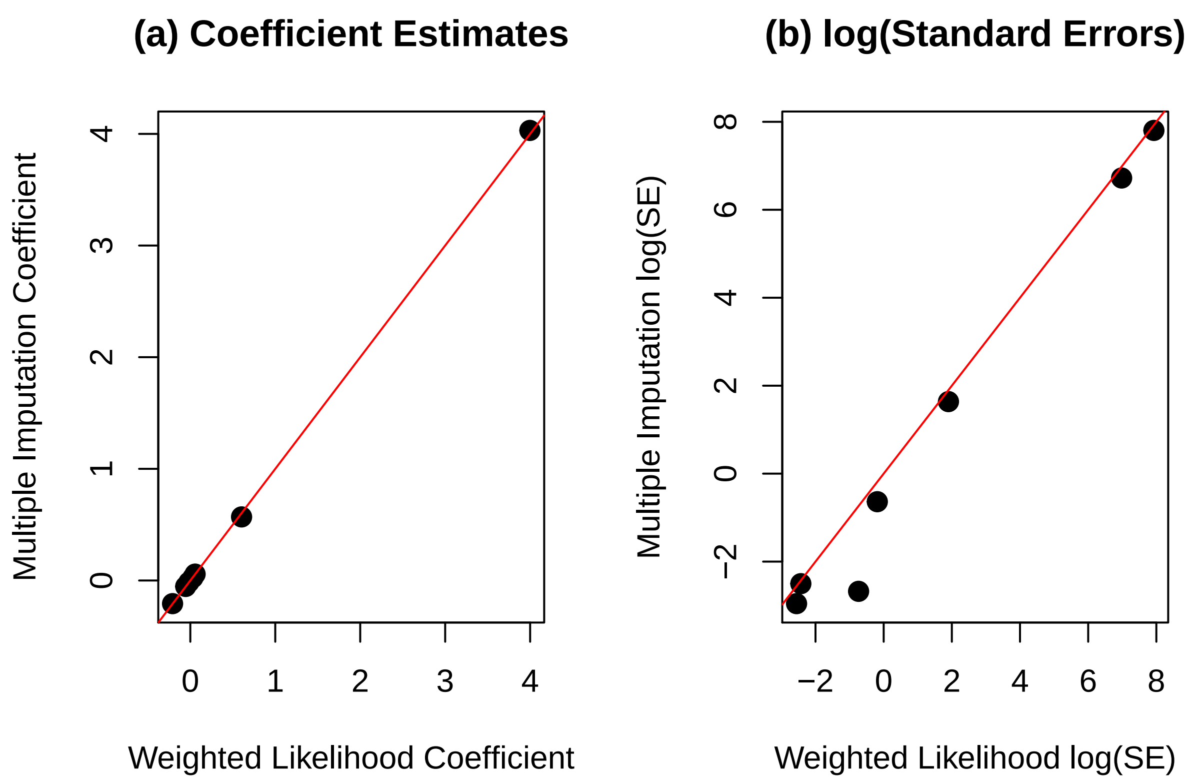


### 7.4 Varying Coefficient Models for Movement

Finally, we show how the SWL lends itself to penalized inference by considering a varying-coefficient model to capture time-varying response to the "distance to rookery" directional covariate (d2r). The SWL makes inference in such a model accessible, as the "gam" function in the 'mgcv' package allows for fitting varying coefficient models in Poisson regression. The code is simple and a straightforward extension of the non-penalized GLM inference.

```
library(mgcv)
```

```
## Loading required package: nlme

##
## Attaching package: 'nlme'

## The following object is masked from 'package:raster':
##
##     getData

## This is mgcv 1.8-7. For overview type 'help("mgcv-package")'.
```

```
fit=gam(z~cha+npp+crw+sst.loc+s(t,by=-d2r),
        weights=rep(1/P,nrow(glm.data)),family="poisson",offset=log(tau),data=glm.data)
summary(fit)
```

```
##
## Family: poisson
## Link function: log
##
## Formula:
## z ~ cha + npp + crw + sst.loc + s(t, by = -d2r)
##
## Parametric coefficients:
##              Estimate Std. Error z value Pr(>|z|)
## (Intercept)   2.90553    0.59000   4.925 8.45e-07 ***
## cha          46.76434 2315.71218   0.020   0.9839
## npp           5.15425    4.94199   1.043   0.2970
## crw           0.53321    0.07343   7.261 3.84e-13 ***
## sst.loc      -0.14137    0.05730  -2.467   0.0136 *
## ---
## Signif. codes:  0 '***' 0.001 '**' 0.01 '*' 0.05 '.' 0.1 ' ' 1
##
## Approximate significance of smooth terms:
##             edf Ref.df Chi.sq p-value
## s(t):-d2r 5.368  6.374  100.1  <2e-16 ***
## ---
## Signif. codes:  0 '***' 0.001 '**' 0.01 '*' 0.05 '.' 0.1 ' ' 1
##
## R-sq.(adj) =  -0.17   Deviance explained = 15.7%
## UBRE = -0.96206  Scale est. = 1         n = 39660
```

```r
plot(fit)
abline(h=0,col="red")
```

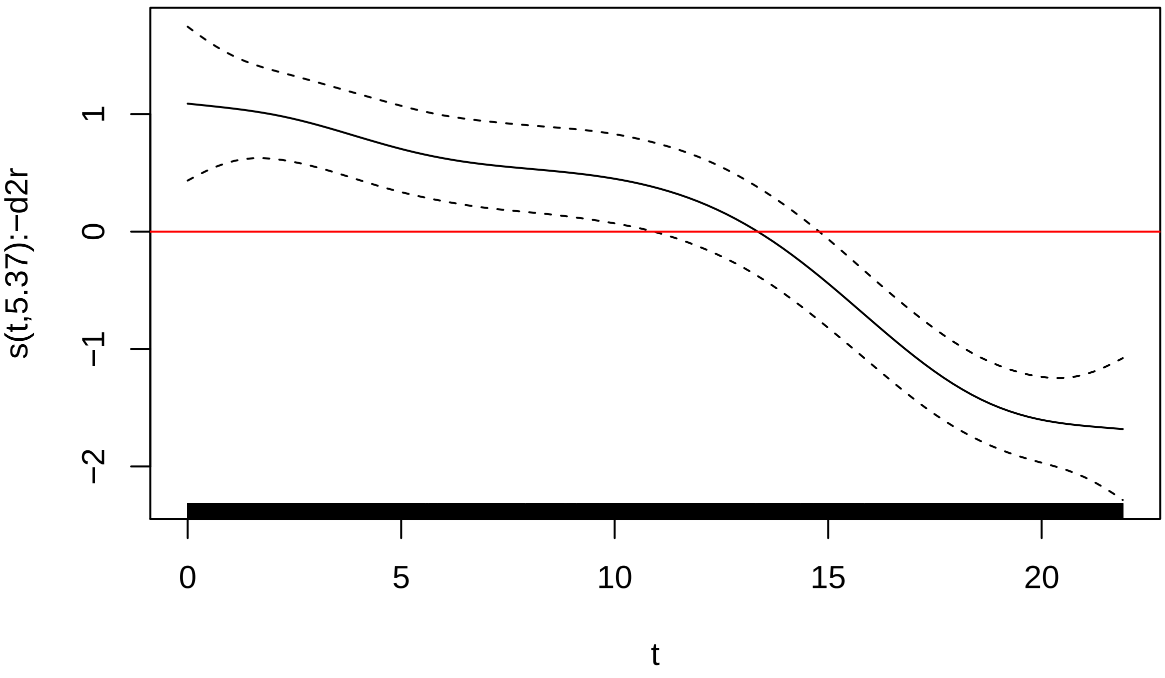


Here we see that the NFS's response to the 'd2r' covariate changes over time, as it is first driven away from the rookery, and then pulled back.
